# Supplementary material for: Dissipation in mesoscale superfluids
Source: arXiv:1704.01968 source file (2017-04-06)
Supplement: Supplementary file 1 [file supp_refs.tex]

\begin{thebibliography}{19}%
\makeatletter
\providecommand \@ifxundefined [1]{%
 \@ifx{#1\undefined}
}%
\providecommand \@ifnum [1]{%
 \ifnum #1\expandafter \@firstoftwo
 \else \expandafter \@secondoftwo
 \fi
}%
\providecommand \@ifx [1]{%
 \ifx #1\expandafter \@firstoftwo
 \else \expandafter \@secondoftwo
 \fi
}%
\providecommand \natexlab [1]{#1}%
\providecommand \enquote  [1]{``#1''}%
\providecommand \bibnamefont  [1]{#1}%
\providecommand \bibfnamefont [1]{#1}%
\providecommand \citenamefont [1]{#1}%
\providecommand \href@noop [0]{\@secondoftwo}%
\providecommand \href [0]{\begingroup \@sanitize@url \@href}%
\providecommand \@href[1]{\@@startlink{#1}\@@href}%
\providecommand \@@href[1]{\endgroup#1\@@endlink}%
\providecommand \@sanitize@url [0]{\catcode `\\12\catcode `\$12\catcode
  `\&12\catcode `\#12\catcode `\^12\catcode `\_12\catcode `\%12\relax}%
\providecommand \@@startlink[1]{}%
\providecommand \@@endlink[0]{}%
\providecommand \url  [0]{\begingroup\@sanitize@url \@url }%
\providecommand \@url [1]{\endgroup\@href {#1}{\urlprefix }}%
\providecommand \urlprefix  [0]{URL }%
\providecommand \Eprint [0]{\href }%
\providecommand \doibase [0]{http://dx.doi.org/}%
\providecommand \selectlanguage [0]{\@gobble}%
\providecommand \bibinfo  [0]{\@secondoftwo}%
\providecommand \bibfield  [0]{\@secondoftwo}%
\providecommand \translation [1]{[#1]}%
\providecommand \BibitemOpen [0]{}%
\providecommand \bibitemStop [0]{}%
\providecommand \bibitemNoStop [0]{.\EOS\space}%
\providecommand \EOS [0]{\spacefactor3000\relax}%
\providecommand \BibitemShut  [1]{\csname bibitem#1\endcsname}%
\let\auto@bib@innerbib\@empty
%</preamble>
\bibitem [{\citenamefont {Morse}\ and\ \citenamefont
  {Feshbach}(1953)}]{SImorsefeshbach}%
  \BibitemOpen
  \bibfield  {author} {\bibinfo {author} {\bibfnamefont {P.M.C.}\ \bibnamefont
  {Morse}}\ and\ \bibinfo {author} {\bibfnamefont {H.}~\bibnamefont
  {Feshbach}},\ }\href@noop {} {\emph {\bibinfo {title} {Methods of Theoretical
  Physics}}},\ Vol.~\bibinfo {volume} {2}\ (\bibinfo  {publisher}
  {McGraw-Hill},\ \bibinfo {year} {1953})\BibitemShut {NoStop}%
\bibitem [{\citenamefont {Blount}\ and\ \citenamefont {Varma}(1976)}]{SIblount}%
  \BibitemOpen
  \bibfield  {author} {\bibinfo {author} {\bibfnamefont {E}~\bibnamefont
  {Blount}}\ and\ \bibinfo {author} {\bibfnamefont {C}~\bibnamefont {Varma}},\
  }\bibfield  {title} {\enquote {\bibinfo {title} {{Hydrodynamics of vortex
  generation in flowing superfluid helium}},}\ }\href@noop {} {\bibfield
  {journal} {\bibinfo  {journal} {Phys. Rev. B}\ }\textbf {\bibinfo {volume}
  {14}},\ \bibinfo {pages} {2888} (\bibinfo {year} {1976})}\BibitemShut
  {NoStop}%
\bibitem [{\citenamefont {Schwarz}(1993)}]{SIschwarz}%
  \BibitemOpen
  \bibfield  {author} {\bibinfo {author} {\bibfnamefont {K~W}\ \bibnamefont
  {Schwarz}},\ }\bibfield  {title} {\enquote {\bibinfo {title} {{Phase slip and
  phase-slip cascades in He4superflow through a small orifice}},}\ }\href@noop
  {} {\bibfield  {journal} {\bibinfo  {journal} {Phys. Rev. Lett.}\ }\textbf
  {\bibinfo {volume} {71}},\ \bibinfo {pages} {259} (\bibinfo {year}
  {1993})}\BibitemShut {NoStop}%
\bibitem [{\citenamefont {Josephson}(1966)}]{SIjosephson}%
  \BibitemOpen
  \bibfield  {author} {\bibinfo {author} {\bibfnamefont {B.~D.}\ \bibnamefont
  {Josephson}},\ }\bibfield  {title} {\enquote {\bibinfo {title} {{Relation
  between the superfluid density and order parameter for superfluid He near
  Tc}},}\ }\href@noop {} {\bibfield  {journal} {\bibinfo  {journal} {Phys.
  Lett.}\ }\textbf {\bibinfo {volume} {21}},\ \bibinfo {pages} {608} (\bibinfo
  {year} {1966})}\BibitemShut {NoStop}%
\bibitem [{\citenamefont {Donnelly}\ and\ \citenamefont
  {Barenghi}(1998)}]{SIDonnelly:1998ge}%
  \BibitemOpen
  \bibfield  {author} {\bibinfo {author} {\bibfnamefont {R~J}\ \bibnamefont
  {Donnelly}}\ and\ \bibinfo {author} {\bibfnamefont {C~F}\ \bibnamefont
  {Barenghi}},\ }\bibfield  {title} {\enquote {\bibinfo {title} {{The observed
  properties of liquid helium at the saturated vapor pressure}},}\ }\href@noop
  {} {\bibfield  {journal} {\bibinfo  {journal} {J. Phys. Chem.}\ }\textbf
  {\bibinfo {volume} {27}},\ \bibinfo {pages} {1217} (\bibinfo {year}
  {1998})}\BibitemShut {NoStop}%
\bibitem [{\citenamefont {Prokof'ev}\ \emph {et~al.}(2004)\citenamefont
  {Prokof'ev}, \citenamefont {Ruebenacker},\ and\ \citenamefont
  {Svistunov}}]{SIProkofev:2004js}%
  \BibitemOpen
  \bibfield  {author} {\bibinfo {author} {\bibfnamefont {Nikolay}\ \bibnamefont
  {Prokof'ev}}, \bibinfo {author} {\bibfnamefont {Oliver}\ \bibnamefont
  {Ruebenacker}}, \ and\ \bibinfo {author} {\bibfnamefont {Boris}\ \bibnamefont
  {Svistunov}},\ }\bibfield  {title} {\enquote {\bibinfo {title} {{Weakly
  interacting Bose gas in the vicinity of the normal-fluid-superfluid
  transition}},}\ }\href {\doibase 10.1103/PhysRevA.69.053625} {\bibfield
  {journal} {\bibinfo  {journal} {Phys. Rev. A}\ }\textbf {\bibinfo {volume}
  {69}},\ \bibinfo {pages} {053625} (\bibinfo {year} {2004})}\BibitemShut
  {NoStop}%
\bibitem [{\citenamefont {Varoquaux}(2015)}]{SIvaroquauxrmp}%
  \BibitemOpen
  \bibfield  {author} {\bibinfo {author} {\bibfnamefont {Eric}\ \bibnamefont
  {Varoquaux}},\ }\bibfield  {title} {\enquote {\bibinfo {title}
  {{Anderson{\textquoteright}s considerations on the flow of superfluid helium:
  Some offshoots}},}\ }\href@noop {} {\bibfield  {journal} {\bibinfo  {journal}
  {Rev. Mod. Phys.}\ }\textbf {\bibinfo {volume} {87}},\ \bibinfo {pages} {803}
  (\bibinfo {year} {2015})}\BibitemShut {NoStop}%
\bibitem [{\citenamefont {Harrison}\ and\ \citenamefont
  {Mendelssohn}(1974)}]{SIharrison}%
  \BibitemOpen
  \bibfield  {author} {\bibinfo {author} {\bibfnamefont {S.~J.}\ \bibnamefont
  {Harrison}}\ and\ \bibinfo {author} {\bibfnamefont {K.}~\bibnamefont
  {Mendelssohn}},\ }\bibfield  {title} {\enquote {\bibinfo {title} {{Superfluid
  4He Velocities in Narrow Channels between 1.8 and 0.3 K}},}\ }in\ \href@noop
  {} {\emph {\bibinfo {booktitle} {Low Temperature Physics}}},\ \bibinfo
  {editor} {edited by\ \bibinfo {editor} {\bibfnamefont {T~D}\ \bibnamefont
  {Timmerhaus}}}\ (\bibinfo  {publisher} {Springer},\ \bibinfo {address} {New
  York},\ \bibinfo {year} {1974})\ p.\ \bibinfo {pages} {298}\BibitemShut
  {NoStop}%
\bibitem [{\citenamefont {Duc}\ \emph {et~al.}(2015)\citenamefont {Duc},
  \citenamefont {Savard}, \citenamefont {Petrescu}, \citenamefont {Rosenow},
  \citenamefont {Del~Maestro},\ and\ \citenamefont {Gervais}}]{SIduc}%
  \BibitemOpen
  \bibfield  {author} {\bibinfo {author} {\bibfnamefont {Pierre-Francois}\
  \bibnamefont {Duc}}, \bibinfo {author} {\bibfnamefont {Michel}\ \bibnamefont
  {Savard}}, \bibinfo {author} {\bibfnamefont {Matei}\ \bibnamefont
  {Petrescu}}, \bibinfo {author} {\bibfnamefont {Bernd}\ \bibnamefont
  {Rosenow}}, \bibinfo {author} {\bibfnamefont {Adrian}\ \bibnamefont
  {Del~Maestro}}, \ and\ \bibinfo {author} {\bibfnamefont {Guillaume}\
  \bibnamefont {Gervais}},\ }\bibfield  {title} {\enquote {\bibinfo {title}
  {{Critical flow and dissipation in a quasi-one-dimensional superfluid}},}\
  }\href@noop {} {\bibfield  {journal} {\bibinfo  {journal} {Science Adv.}\
  }\textbf {\bibinfo {volume} {1}},\ \bibinfo {pages} {e1400222} (\bibinfo
  {year} {2015})}\BibitemShut {NoStop}%
\bibitem [{\citenamefont {Neely}\ \emph {et~al.}(2010)\citenamefont {Neely},
  \citenamefont {Samson}, \citenamefont {Bradley}, \citenamefont {Davis},\ and\
  \citenamefont {Anderson}}]{SIneely}%
  \BibitemOpen
  \bibfield  {author} {\bibinfo {author} {\bibfnamefont {T.~W.}\ \bibnamefont
  {Neely}}, \bibinfo {author} {\bibfnamefont {E.~C.}\ \bibnamefont {Samson}},
  \bibinfo {author} {\bibfnamefont {A.~S.}\ \bibnamefont {Bradley}}, \bibinfo
  {author} {\bibfnamefont {M.~J.}\ \bibnamefont {Davis}}, \ and\ \bibinfo
  {author} {\bibfnamefont {B.~P.}\ \bibnamefont {Anderson}},\ }\bibfield
  {title} {\enquote {\bibinfo {title} {{Observation of Vortex Dipoles in an
  Oblate Bose-Einstein Condensate}},}\ }\href@noop {} {\bibfield  {journal}
  {\bibinfo  {journal} {Phys. Rev. Lett.}\ }\textbf {\bibinfo {volume} {104}},\
  \bibinfo {pages} {160401} (\bibinfo {year} {2010})}\BibitemShut {NoStop}%
\bibitem [{\citenamefont {Ramanathan}\ \emph {et~al.}(2011)\citenamefont
  {Ramanathan}, \citenamefont {Wright}, \citenamefont {Muniz}, \citenamefont
  {Zelan}, \citenamefont {Hill}, \citenamefont {Lobb}, \citenamefont
  {Helmerson}, \citenamefont {Phillips},\ and\ \citenamefont
  {Campbell}}]{SIramanathan}%
  \BibitemOpen
  \bibfield  {author} {\bibinfo {author} {\bibfnamefont {A.}~\bibnamefont
  {Ramanathan}}, \bibinfo {author} {\bibfnamefont {K.~C.}\ \bibnamefont
  {Wright}}, \bibinfo {author} {\bibfnamefont {S.~R.}\ \bibnamefont {Muniz}},
  \bibinfo {author} {\bibfnamefont {M.}~\bibnamefont {Zelan}}, \bibinfo
  {author} {\bibfnamefont {W.~T.}\ \bibnamefont {Hill}}, \bibinfo {author}
  {\bibfnamefont {C.~J.}\ \bibnamefont {Lobb}}, \bibinfo {author}
  {\bibfnamefont {K.}~\bibnamefont {Helmerson}}, \bibinfo {author}
  {\bibfnamefont {W.~D.}\ \bibnamefont {Phillips}}, \ and\ \bibinfo {author}
  {\bibfnamefont {G.~K.}\ \bibnamefont {Campbell}},\ }\bibfield  {title}
  {\enquote {\bibinfo {title} {{Superflow in a Toroidal Bose-Einstein
  Condensate: An Atom Circuit with a Tunable Weak Link}},}\ }\href@noop {}
  {\bibfield  {journal} {\bibinfo  {journal} {Phys. Rev. Lett.}\ }\textbf
  {\bibinfo {volume} {106}},\ \bibinfo {pages} {130401} (\bibinfo {year}
  {2011})}\BibitemShut {NoStop}%
\bibitem [{\citenamefont {Raman}\ \emph {et~al.}(1999)\citenamefont {Raman},
  \citenamefont {K{\"o}hl}, \citenamefont {Onofrio}, \citenamefont {Durfee},
  \citenamefont {Kuklewicz}, \citenamefont {Hadzibabic},\ and\ \citenamefont
  {Ketterle}}]{SIraman}%
  \BibitemOpen
  \bibfield  {author} {\bibinfo {author} {\bibfnamefont {C.}~\bibnamefont
  {Raman}}, \bibinfo {author} {\bibfnamefont {M.}~\bibnamefont {K{\"o}hl}},
  \bibinfo {author} {\bibfnamefont {R.}~\bibnamefont {Onofrio}}, \bibinfo
  {author} {\bibfnamefont {D.~S.}\ \bibnamefont {Durfee}}, \bibinfo {author}
  {\bibfnamefont {C.~E.}\ \bibnamefont {Kuklewicz}}, \bibinfo {author}
  {\bibfnamefont {Z.}~\bibnamefont {Hadzibabic}}, \ and\ \bibinfo {author}
  {\bibfnamefont {W.}~\bibnamefont {Ketterle}},\ }\bibfield  {title} {\enquote
  {\bibinfo {title} {{Evidence for a Critical Velocity in a Bose-Einstein
  Condensed Gas}},}\ }\href@noop {} {\bibfield  {journal} {\bibinfo  {journal}
  {Phys. Rev. Lett.}\ }\textbf {\bibinfo {volume} {83}},\ \bibinfo {pages}
  {2502} (\bibinfo {year} {1999})}\BibitemShut {NoStop}%
\bibitem [{\citenamefont {Weimer}\ \emph {et~al.}(2015)\citenamefont {Weimer},
  \citenamefont {Morgener}, \citenamefont {Singh}, \citenamefont {Siegl},
  \citenamefont {Hueck}, \citenamefont {Luick}, \citenamefont {Mathey},\ and\
  \citenamefont {Moritz}}]{SIweimer}%
  \BibitemOpen
  \bibfield  {author} {\bibinfo {author} {\bibfnamefont {Wolf}\ \bibnamefont
  {Weimer}}, \bibinfo {author} {\bibfnamefont {Kai}\ \bibnamefont {Morgener}},
  \bibinfo {author} {\bibfnamefont {Vijay~Pal}\ \bibnamefont {Singh}}, \bibinfo
  {author} {\bibfnamefont {Jonas}\ \bibnamefont {Siegl}}, \bibinfo {author}
  {\bibfnamefont {Klaus}\ \bibnamefont {Hueck}}, \bibinfo {author}
  {\bibfnamefont {Niclas}\ \bibnamefont {Luick}}, \bibinfo {author}
  {\bibfnamefont {Ludwig}\ \bibnamefont {Mathey}}, \ and\ \bibinfo {author}
  {\bibfnamefont {Henning}\ \bibnamefont {Moritz}},\ }\bibfield  {title}
  {\enquote {\bibinfo {title} {{Critical Velocity in the BEC-BCS Crossover}},}\
  }\href@noop {} {\bibfield  {journal} {\bibinfo  {journal} {Phys. Rev. Lett.}\
  }\textbf {\bibinfo {volume} {114}},\ \bibinfo {pages} {095301} (\bibinfo
  {year} {2015})}\BibitemShut {NoStop}%
\bibitem [{\citenamefont {Chien}\ \emph {et~al.}(2015)\citenamefont {Chien},
  \citenamefont {Peotta},\ and\ \citenamefont {Di~Ventra}}]{SIchien}%
  \BibitemOpen
  \bibfield  {author} {\bibinfo {author} {\bibfnamefont {Chih-Chun}\
  \bibnamefont {Chien}}, \bibinfo {author} {\bibfnamefont {Sebastiano}\
  \bibnamefont {Peotta}}, \ and\ \bibinfo {author} {\bibfnamefont
  {Massimiliano}\ \bibnamefont {Di~Ventra}},\ }\bibfield  {title} {\enquote
  {\bibinfo {title} {{Quantum transport in ultracold atoms}},}\ }\href@noop {}
  {\bibfield  {journal} {\bibinfo  {journal} {Nature Phys.}\ }\textbf {\bibinfo
  {volume} {11}},\ \bibinfo {pages} {998} (\bibinfo {year} {2015})}\BibitemShut
  {NoStop}%
\bibitem [{\citenamefont {Capogrosso-Sansone}\ \emph
  {et~al.}(2010)\citenamefont {Capogrosso-Sansone}, \citenamefont {Giorgini},
  \citenamefont {Pilati}, \citenamefont {Pollet}, \citenamefont {Prokof'ev},
  \citenamefont {Svistunov},\ and\ \citenamefont
  {Troyer}}]{SICapogrossoSansone:2010kt}%
  \BibitemOpen
  \bibfield  {author} {\bibinfo {author} {\bibfnamefont {B}~\bibnamefont
  {Capogrosso-Sansone}}, \bibinfo {author} {\bibfnamefont {S}~\bibnamefont
  {Giorgini}}, \bibinfo {author} {\bibfnamefont {S.}~\bibnamefont {Pilati}},
  \bibinfo {author} {\bibfnamefont {L}~\bibnamefont {Pollet}}, \bibinfo
  {author} {\bibfnamefont {N}~\bibnamefont {Prokof'ev}}, \bibinfo {author}
  {\bibfnamefont {B}~\bibnamefont {Svistunov}}, \ and\ \bibinfo {author}
  {\bibfnamefont {M.}~\bibnamefont {Troyer}},\ }\bibfield  {title} {\enquote
  {\bibinfo {title} {{The Beliaev technique for a weakly interacting Bose
  gas}},}\ }\href@noop {} {\bibfield  {journal} {\bibinfo  {journal} {New J.
  Phys.}\ }\textbf {\bibinfo {volume} {12}},\ \bibinfo {pages} {043010}
  (\bibinfo {year} {2010})}\BibitemShut {NoStop}%
\bibitem [{\citenamefont {Langer}\ and\ \citenamefont {Fisher}(1967)}]{SIlanger}%
  \BibitemOpen
  \bibfield  {author} {\bibinfo {author} {\bibfnamefont {J.}~\bibnamefont
  {Langer}}\ and\ \bibinfo {author} {\bibfnamefont {Michael}\ \bibnamefont
  {Fisher}},\ }\bibfield  {title} {\enquote {\bibinfo {title} {{Intrinsic
  Critical Velocity of a Superfluid}},}\ }\href@noop {} {\bibfield  {journal}
  {\bibinfo  {journal} {Phys. Rev. Lett.}\ }\textbf {\bibinfo {volume} {19}},\
  \bibinfo {pages} {560} (\bibinfo {year} {1967})}\BibitemShut {NoStop}%
\bibitem [{\citenamefont {Singasaas}\ and\ \citenamefont
  {Ahlers}(1984)}]{SISiAh84}%
  \BibitemOpen
  \bibfield  {author} {\bibinfo {author} {\bibfnamefont {Alan}\ \bibnamefont
  {Singasaas}}\ and\ \bibinfo {author} {\bibfnamefont {Guenter}\ \bibnamefont
  {Ahlers}},\ }\bibfield  {title} {\enquote {\bibinfo {title} {{Universality of
  static properties near the superfluid transition in He4}},}\ }\href@noop {}
  {\bibfield  {journal} {\bibinfo  {journal} {Phys. Rev. B}\ }\textbf {\bibinfo
  {volume} {30}},\ \bibinfo {pages} {5103} (\bibinfo {year}
  {1984})}\BibitemShut {NoStop}%
\bibitem [{\citenamefont {Langer}\ and\ \citenamefont {Ambegaokar}(1967)}]{SILA}%
  \BibitemOpen
  \bibfield  {author} {\bibinfo {author} {\bibfnamefont {J.}~\bibnamefont
  {Langer}}\ and\ \bibinfo {author} {\bibfnamefont {Vinay}\ \bibnamefont
  {Ambegaokar}},\ }\bibfield  {title} {\enquote {\bibinfo {title} {{Intrinsic
  Resistive Transition in Narrow Superconducting Channels}},}\ }\href@noop {}
  {\bibfield  {journal} {\bibinfo  {journal} {Phys. Rev.}\ }\textbf {\bibinfo
  {volume} {164}},\ \bibinfo {pages} {498} (\bibinfo {year}
  {1967})}\BibitemShut {NoStop}%
\bibitem [{\citenamefont {McCumber}\ and\ \citenamefont {Halperin}(1970)}]{SIMH}%
  \BibitemOpen
  \bibfield  {author} {\bibinfo {author} {\bibfnamefont {D.}~\bibnamefont
  {McCumber}}\ and\ \bibinfo {author} {\bibfnamefont {B.}~\bibnamefont
  {Halperin}},\ }\bibfield  {title} {\enquote {\bibinfo {title} {{Time Scale of
  Intrinsic Resistive Fluctuations in Thin Superconducting Wires}},}\
  }\href@noop {} {\bibfield  {journal} {\bibinfo  {journal} {Phys. Rev. B}\
  }\textbf {\bibinfo {volume} {1}},\ \bibinfo {pages} {1054} (\bibinfo {year}
  {1970})}\BibitemShut {NoStop}%
\end{thebibliography}%
